# Supplementary material for: Holistic Utility Preference Learning for Listwise Alignment
Source: arXiv:2410.18127 source file (2025-12-16)
Supplement: Supplementary file 1 [file appendix.tex]

% \section*{\centering \LARGE{Appendix}}
% \tableofcontents

% \section{Detail Limitations}
% \addcontentsline{apc}{section}{\textnormal{B: Limitations}}

% In conducting our experiments, we adhere to benchmarks that are widely recognized and routinely utilized in the literature on human preference alignment. It is important to note, however, that despite our best efforts, there remain certain unavoidable limitations that merit consideration. In the process of constructing a ranking preference dataset, we employ a reward model to serve as a proxy for human evaluations. While the reward model we employ achieves a high level of accuracy, it is important to acknowledge that there might still be subtle discrepancies when compared to human evaluations. In the future, we are also interested in exploring more high-quality reward models as proxies for human evaluations. 

\section{Detailed Sorting Process in Sorting Networks}
\label{sec:sorting_detail}

This work leverages the odd-even sorting network algorithm. As depicted in Figure \ref{fig:diff_sort}, an ordered sequence of $K$ elements can be achieved through a $K\text{-layer}$ sorting network. Each layer of the odd-even sorting network operates by comparing and swapping \textit{adjacent elements} at either odd or even indices, thereby organizing them in a desired order. The process alternates between odd and even stages. During the odd stage, all pairs of elements at odd indices (i.e., positions 1 and 2, 3 and 4, 5 and 6, etc.) are compared and swapped if necessary according to the desired order. In the even stage, all pairs of elements at even indices (i.e., positions 2 and 3, 4 and 5, 6 and 7, etc.) are compared and swapped according to the desired order.

To illustrate this mechanism, consider an unordered sequence $(10, 2, 4, 8)$ with length $K=4$ that we wish to arrange in descending order. The sorting process proceeds through alternating phases as follows:

\begin{itemize}
\item The first iteration (even phase) begins with indices $0$ and $2$, corresponding to values $(10, 4)$. These elements are compared with their subsequent elements $(2, 8)$ respectively. Since $10 > 2$ satisfies the descending order requirement, no swap is needed for the first pair. However, $4 < 8$ violates the descending order requirement, so $4$ and $8$ are swapped. This phase yields an intermediate sequence $(10, 2, 8, 4)$. 

\item The second iteration (odd phase) focuses on indices $1$ and $3$, corresponding to elements $(2, 8)$. The element $2$ is compared with its subsequent element $8$, and since $2 < 8$, they are swapped. The element at index $3$ has no subsequent element for comparison, thus remaining unchanged. This phase transforms the sequence to $(10, 8, 2, 4)$. 

\item In the third iteration (even phase), indices $0$ and $2$ are examined. At index $0$, since $10 > 8$, no swap is needed. At index $2$, comparing $2$ with $4$, since $2 < 4$, they are swapped. Upon reaching a sequence satisfying the descending-order property $(10, 8, 4, 2)$, the algorithm terminates.
\end{itemize}

\begin{wrapfigure}{h}{0.32\textwidth}
    \vspace{-1em}
    \centering
    \includegraphics[width=0.32\columnwidth]{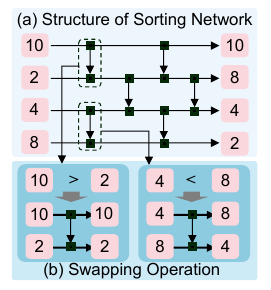}
    % \vspace{-0.1em}
    \caption{Sort $\mathbf{s}=(10,2,4,8)$ in descending order using a sorting network. (a) The structure of the sorting network; (b) the swapping operation in the first layer. }
    \label{fig:diff_sort}
    \vspace{-0.25em}
\end{wrapfigure}

As illustrated in Section \ref{sec:diff_swap_op}, this sorting operation can also be represented using permutation matrices. In our sorting process, the corresponding permutation matrices for each iteration are:
\begin{equation*}
    \mathbf{P}_1 = \begin{bmatrix}
    1 & 0 & 0 & 0 \\
    0 & 1 & 0 & 0 \\
    0 & 0 & 0 & 1 \\
    0 & 0 & 1 & 0
    \end{bmatrix}, \quad
    \mathbf{P}_2 = \begin{bmatrix}
    1 & 0 & 0 & 0 \\
    0 & 0 & 1 & 0 \\
    0 & 1 & 0 & 0 \\
    0 & 0 & 0 & 1
    \end{bmatrix}, \quad
    \mathbf{P}_3 = \begin{bmatrix}
    1 & 0 & 0 & 0 \\
    0 & 1 & 0 & 0 \\
    0 & 0 & 0 & 1 \\
    0 & 0 & 1 & 0
    \end{bmatrix}
\end{equation*}
Therefore, starting with initial sequence $\mathbf{s}_0 = [10, 2, 4, 8]^\top$, each layer's result can be represented through matrix multiplication: $\mathbf{s}_1 = \mathbf{P}_1^{\top} \cdot \mathbf{s}_0, \quad \mathbf{s}_2 = \mathbf{P}_2^{\top} \cdot \mathbf{s}_1, \quad \mathbf{s}_3 = \mathbf{P}_3^{\top} \cdot \mathbf{s}_2$. We can also obtain the complete sorting process's permutation matrix as follows:
\begin{equation*}
    \mathbf{P} = \mathbf{P}_1 \cdot \mathbf{P}_2 \cdot \mathbf{P}_3 = \begin{bmatrix}
    1 & 0 & 0 & 0 \\
    0 & 0 & 1 & 0 \\
    0 & 0 & 0 & 1 \\
    0 & 1 & 0 & 0
    \end{bmatrix}
\end{equation*}
The final ordered sequence is therefore given by:
\begin{equation*}
    \mathbf{s}_{\text{order}} = \mathbf{P}^{\top} \cdot \mathbf{s} = [10, 8, 4, 2]^\top.
\end{equation*}

\section{Construction the Ranking Preference Data}
% \addcontentsline{apc}{section}{\textnormal{D: Construction the Ranking Preference Data.} } 
\label{appendix:rankhh}
% Datasets. Anthropic’s Helpful and Harmless (HH) [Bai et al., 2022] contains 161k/8.5k train-245
% ing/test samples. Each sample consists of a prompt and a pair of responses (chosen and reject),246
% where “chosen" represents the preferred response and “reject" represents the less preferred response.247
% We also generate additional responses for each prompt and rate each response using a reward model248
% DeBERTa2, resulting in ranking preference data of a list size K = 8. For more details, please refer249
% to Appendix C.

\textbf{HH Dataset.} To construct ranking preference data based on \textbf{HH} dataset, we first supervised fine-tune(SFT) the Qwen1.5-4B model with \textbf{HH} dataset. Subsequently, we sample $K=6$ responses for each prompt $x^i$ in \textbf{HH} dataset using trained SFT model (Qwen1.5-4B) with parameter $temperature = 0.7, top\_k = 40$. We combine the sampled data and the original pairwise data to obtain the $K=8$ responses. We then score each response with a reward model $R$. In our work, we use the RM-Deberta-v3-large-v2\footnotemark[\value{footnote}] model as our reward model, which is based on the DeBERTaV3 \cite{DBLP:conf/iclr/HeLGC21}, subsequently trained on the HH dataset. 

Specifically, following \cite{liu2024lipo}, we compute the score $s^i_j$ of each response $y^i_j$ with respect to the prompt $x^i$ as follows:
\begin{equation*}
s^i_{j} = \frac{1}{K} \sum_{l=1}^{K} \frac{e^{R(x^{i},y^i_{j})}}{e^{R(x^{i},y^i_{j})} + e^{R(x^{i},y^i_{l})}}, \text{where} ~ R ~ \text{is a reward model}.
\label{sig_func}
\end{equation*}

Based on the discussion above, we can construct our ranking preference dataset as $D = \{x^i, \mathbf{y}^i, \mathbf{s}^i\}_{i=1}^N$, where $\mathbf{y}^i = (y^i_1,...,y^i_K)$ and $ \mathbf{s}^i 
= (s^i_1,...,s^i_K)$. To support conducting an ablation study on the size $K$ of the ranking preference dataset, we also split this dataset of size $K=8$ into three subsets, each with sizes $K=2$, $K=4$, and $K=6$, respectively. We also provide an example of our ranking preference dataset as shown in Table \ref{tab:example-hhrank}.

\textbf{UltraFeedback Dataset.} This dataset itself contains four responses and corresponding scores, which can be directly used to construct a ranking preference dataset of size $K=4$. We simply normalize these scores to the range $[0,1]$.

\textbf{VLFeedback Dataset.} Similar to the UltraFeedback Dataset, this dataset can be used directly as a ranking preference dataset of size $K=4$. We simply normalize these scores to the range $[0,1]$.

\input{tables/example-rankhh}

\section{Details of Adaptive Rank Policy Scores}
\addcontentsline{apc}{section}{\textnormal{H: Details of Adaptive Rank Policy Scores}}

In our scoring design, we introduce a ranking position-dependent term $\gamma(y)$ to regulate score differences during the differentiable sorting of responses. Specifically, in our score function (Eq.~\ref{eq:gamma_y_2}), the ranking-aware margin between positions $i$ and $j$ is computed as:
\begin{equation*}
    \gamma(y_i)-\gamma(y_j) = \tau \cdot (q(y_i)-q(y_j)) - \beta \cdot ({V}_{q(y_i)}  -  {V}_{q(y_j)})
\end{equation*}
This margin comprises two components: a static term determined by the relative ranking positions $q(y)$, scaled by $\tau$, and a dynamic term controlled by position-specific values ${V}_{q(y)}$, scaled by $\beta$.

For the base margin, we design $q(y_i)-q(y_j)$ based on two key principles: (1) higher-ranked elements (sorted by labeled scores) should be more preferred, and (2) adjacent elements should have smaller score differences. By incorporating the relative positions into the margin calculation, the resulting margin automatically adjusts according to the distance between ranking positions. 

For the dynamic component, we employ $V_{q(y)}$ to track score variations of responses at different ranking positions. When $V_{q(y)}$ increases for higher-ranked responses, the effective margin expands beyond the base margin, enhancing the distinction between responses. Conversely, when score differences narrow, the dynamic component contracts to enable finer differentiation.

Furthermore, to prevent performance degradation of the ARPS scoring scheme caused by drastic variations in ${V}_{q(y)}$ across different instances, we clip the $\log \pi_\theta(y \mid x) / {|y|}$ during updates using a predefined threshold.

\section{Additional Experiments Results}
% \addcontentsline{apc}{section}{\textnormal{G: Additional Experiments Results}}

\subsection{Additional DiffNDCG Discounts Experiments}
\addcontentsline{apc}{subsection}{\textnormal{G.2: Additional DiffNDCG Discounts Experiments}}

To further analyze the impact of discount factors on our diffNDCG metric, we conducted experiments using various diffNDCG variants, including diffNDCG with Adaptive Rank Policy Score and with Policy Reference Ratio Score. We systematically evaluated the impact of varying discount factors across these diffNDCG variants and report results in Table \ref{tab:full_ndcg_discounts}.

We discovered that various discount factors are indeed effective. Among the various discount factors examined, the inverse logarithmic discount and the inverse discount of ranking position emerged as particularly well-balanced choices. These methods offer an effective compromise between emphasizing top-ranked responses and appropriately penalizing their misplacements. We hypothesize that this balance may be attributed to the characteristics of these discount factors: excessively steep discount factors might lead models to entirely disregard lower-ranked responses, while overly gradual discount factors may fail to adequately penalize misplacements based on ranking position.

\label{sec:add_diffndcg_discounts}

\begin{table}[h]
\begin{center}
\caption{A comprehensive comparison of discount factors across various metrics.}
\label{tab:full_ndcg_discounts} 
\resizebox{0.95\linewidth}{!}{%
    \begin{tabular}{l ccc | ccc }
    \toprule
    \multicolumn {1}{l}{ \bf { Methods}}  
    &\multicolumn{3}{c|}{\bf {DRPO w/o ARP}}
    &\multicolumn{3}{c}{\bf {DRPO}}\\
    \bf Discounts  
            &\small{GPT-4 Win Rate}$\uparrow$ 
            &\small{RM Win Rate (vs Chosen)}$\uparrow$ 
            &\small{RM Win Rate (vs SFT)}$\uparrow$   
            &\small{GPT-4 Win Rate}$\uparrow$
            &\small{RM Win Rate (vs Chosen)}$\uparrow$ 
            &\small{RM Win Rate (vs SFT)}$\uparrow$
            \\
    \midrule
    $1/{\sqrt{r}}$  & 36.17\%($\pm$3.33)  & 52.73\%($\pm$3.15)  & 75.58\%($\pm$2.61)
                    & 40.53\%($\pm$4.36)  & 59.17\%($\pm$2.36)  & 79.29\%($\pm$2.89) \\
    
    $1/{\mathrm{log}(1+r)}$ 
                    & 38.30\%($\pm$3.35)  & 53.91\%($\pm$1.46)  & 73.44\%($\pm$3.17)
                    & 42.80\%($\pm$5.01)  & 58.40\%($\pm$2.94)  & 79.88\%($\pm$3.72) \\ 
                    
    $1/r$           & 38.88\%($\pm$4.34)  & 53.32\%($\pm$1.69)  & 74.80\%($\pm$3.88)
                    & 43.37\%($\pm$5.14)  & 56.64\%($\pm$1.29)  & 78.32\%($\pm$2.94) \\
        
    $1/{r^2}$       & 38.02\%($\pm$5.28)  & 52.92\%($\pm$2.78)  & 74.61\%($\pm$1.17)
                    & 40.37\%($\pm$4.17)  & 59.37\%($\pm$0.02)  & 79.30\%($\pm$3.38) \\

    \bottomrule
    \end{tabular}
}
\end{center}
\end{table}

\subsection{Reward Distribution on HH Dataset}
\addcontentsline{apc}{subsection}{\textnormal{G.1: Reward Distribution on HH Dataset}}

\label{sec:reward_distribution}
We also verify our method by comparing the reward distribution of responses. We train Qwen1.5-0.5B and Qwen1.5-1.8B models on the HH dataset using various methods. We then utilize trained models to generate responses according to the prompts within the test split of the HH dataset and score them with a reward model. As Figure \ref{fig:hh-reward-distribution} shows, all methods tend to increase the expected reward. However, our method achieves a greater increase, surpassing multiple methods including LiPO, DPO\textsubscript{BT}, DPO\textsubscript{PL}, and others.

\begin{figure}[htbp]
  \centering
  \begin{minipage}[b]{0.48\textwidth}
    \centering
    \includegraphics[width=\textwidth]{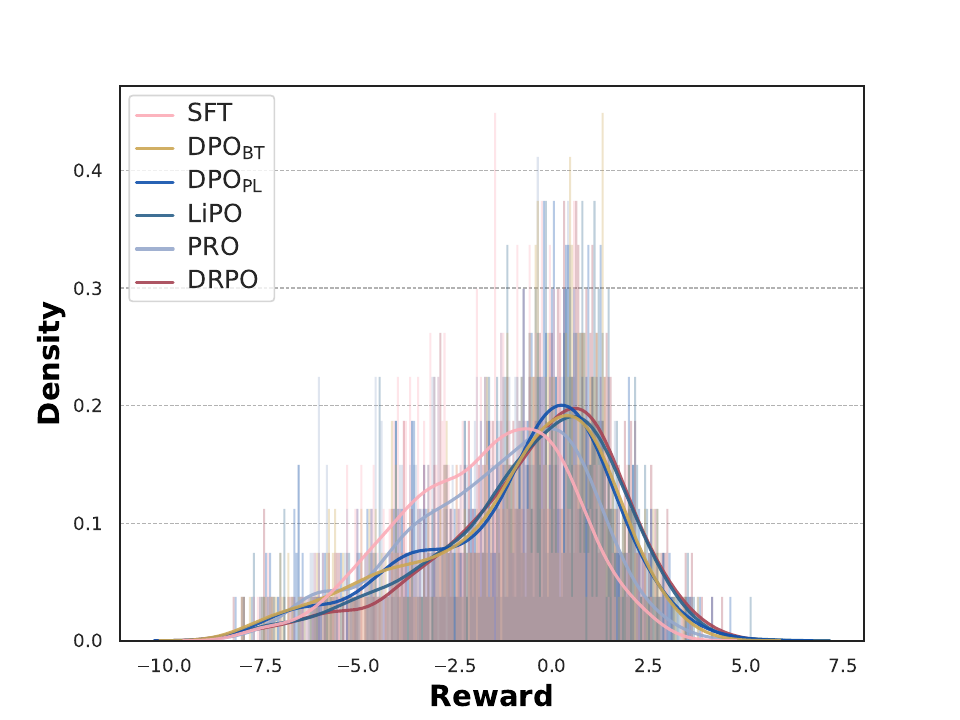}
  \end{minipage}
  \hfill % 该命令添加一些水平空间
  \begin{minipage}[b]{0.48\textwidth}
    \centering
    \includegraphics[width=\textwidth]{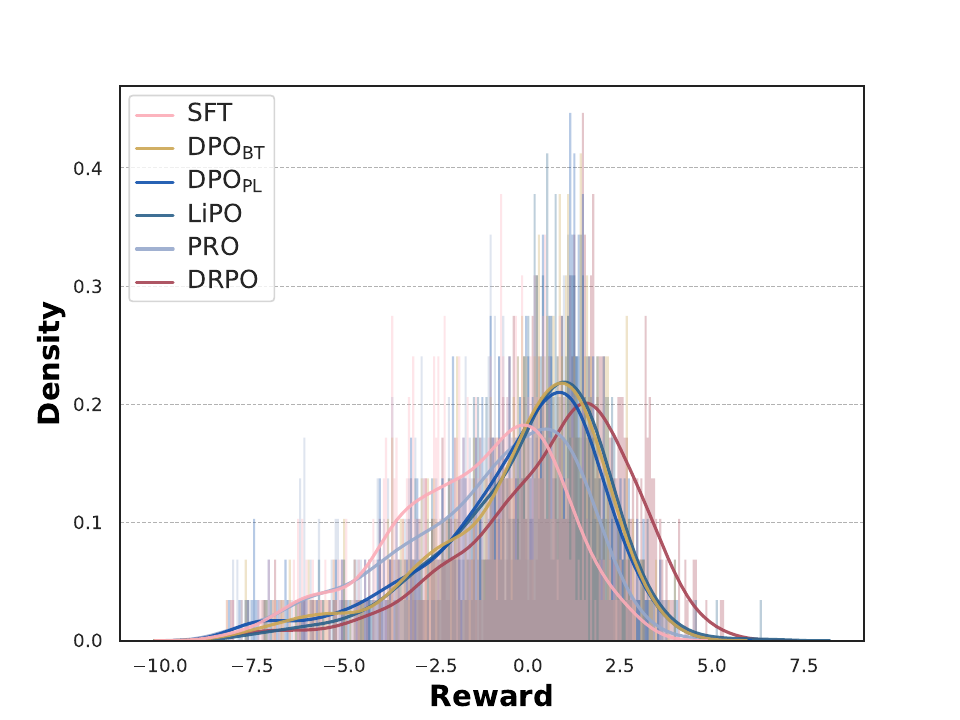}
  \end{minipage}
  \caption{Analysis of reward distribution on the test split of the HH dataset. We train Qwen1.5-0.5B (\textbf{Left}) and Qwen1.5-1.8B (\textbf{Right}) with various methods and compare the reward distribution of responses generated by trained models.}
  \label{fig:hh-reward-distribution}
\end{figure}

\subsection{Experiments on the correlation between NDCG and Win Rate}
% \addcontentsline{apc}{subsection}{\textnormal{G.3: Additional Experiments on the correlation between NDCG and Win Rate}}
\label{sec:add_ndcg_agreement}

To analyze the correlation between NDCG and evaluation metrics such as win rates, we extracted checkpoints during the training and quantified multiple metrics, including NDCG, RM Win Rate, and Ranking Accuracy.

\textbf{Experimental Setup.} Following \cite{chen2024preference}, we analyzed both NDCG and ranking accuracy in relation to win rate using checkpoints collected at different training stages (0\%--100\%) of Qwen1.5-0.5B and Qwen1.5-1.8B. Both models were trained on our constructed ranking preference dataset with sequence length $K=8$. During the training process, we computed NDCG and ranking accuracy metrics, while win rate was evaluated separately using saved model checkpoints. For evaluation metrics, we employed the NDCG implementation from the Allrank\footnote{Available at: \url{https://github.com/allegro/allRank}} framework. For win rate evaluation, we follow the standard experimental setup. The pairwise ranking accuracy between predicted scores $\hat{\mathbf{s}}_{\theta}$ and ground-truth scores $\mathbf{s}$ was computed as:
\begin{equation}
    \text{Accuracy}(\hat{\mathbf{s}}_{\theta}, \mathbf{s}) = \mathbb{E}_{(i,j):1\leq i<j\leq n} [\mathds{1}(\hat{s}_{\theta,i} > \hat{s}_{\theta,j}) = \mathds{1}(s_i > s_j)].
\end{equation}
\textbf{Experimental Results.} The empirical results are visualized in Figure \ref{fig:ndcg-winrate}, with detailed agreement analysis between metrics presented in Table \ref{tab:correlation_ndcg_winrate}. To systematically analyze the relationships between different evaluation metrics, we employ the Pearson correlation coefficient \cite{sedgwick2012pearson}. This coefficient quantifies the linear relationship between metrics, ranging from -1 to 1, where the extremes indicate perfect negative or positive correlations. The statistical significance is assessed using p-values. The results demonstrate strong correlations between NDCG and other evaluation metrics, particularly win rate and ranking accuracy. This high level of agreement suggests that optimizing NDCG effectively improves both win rate and ranking precision, validating the effectiveness of our optimized diffNDCG approach.
\begin{figure}[t]
    \centering
    \subfigure[]{
        \includegraphics[width=0.3\textwidth]{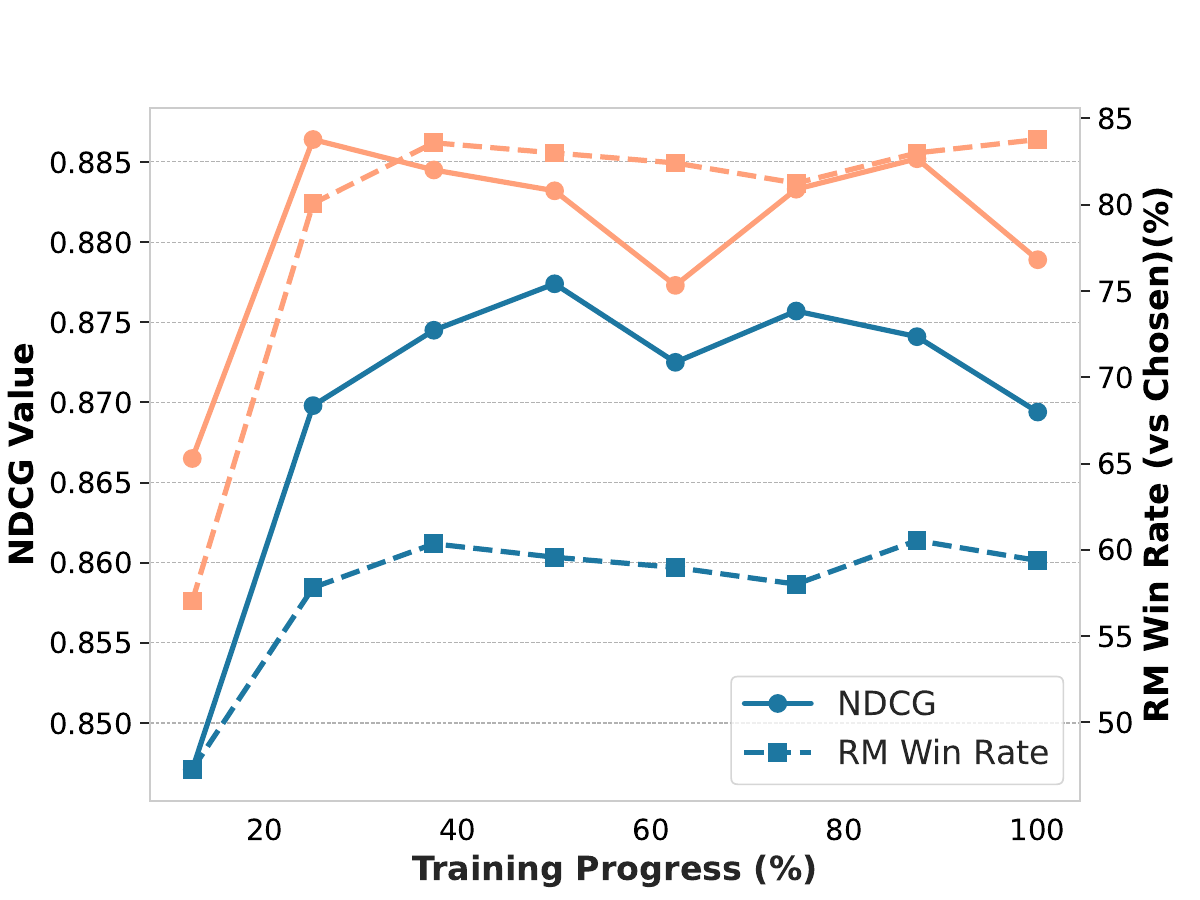}
    }
    \hfill
    \subfigure[]{
        \includegraphics[width=0.3\textwidth]{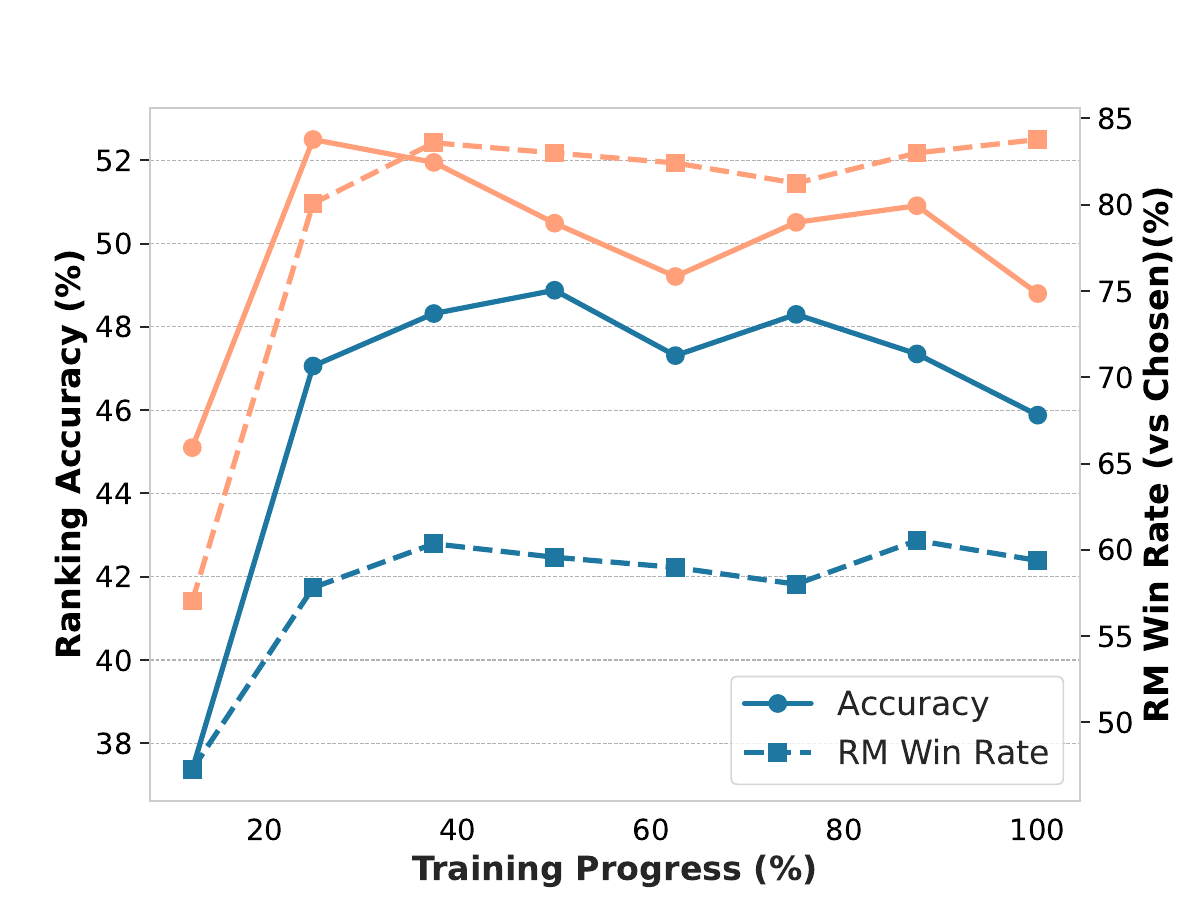}
    }
    \hfill
    \subfigure[]{
        \includegraphics[width=0.3\textwidth]{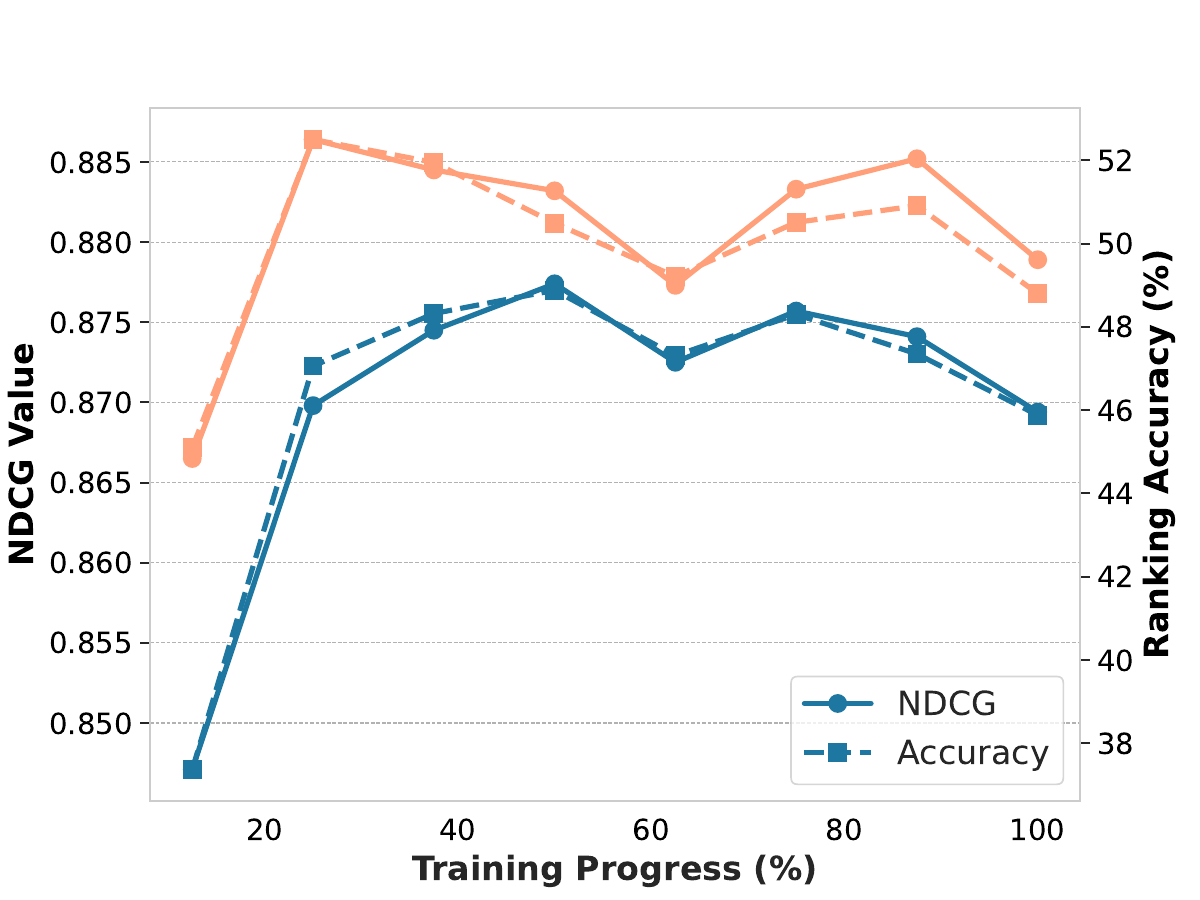}
    }
    \caption{Relationships among Win Rate, NDCG, and Accuracy during training for two models: Qwen 1.5-0.5B (\textcolor{blue}{\textbf{blue}}) and Qwen 1.5-1.8B (\textcolor{orange}{\textbf{orange}}) when using DRPO. (a) NDCG versus RM Win Rate, (b) Ranking Accuracy versus RM Win Rate, and (c) NDCG versus Ranking Accuracy.}
    \label{fig:ndcg-winrate}
\end{figure}

\begin{table}[t]
\begin{center}
\caption{Agreement between different metrics.}
\label{tab:correlation_ndcg_winrate} 
\resizebox{0.6\textwidth}{!}{%
    \begin{tabular}{l c  c }
    \toprule
    \textbf{Metrics} & \textbf{Agreement} & \textbf{P-Value} \\
    \midrule
    \multicolumn{3}{c}{ {Qwen1.5-0.5B-DRPO}}\\
    \midrule
    NDCG \& RM Win Rate             & 0.9522 & 0.00026 \\
    Ranking Accuracy \& RM Win Rate & 0.9493 & 0.00031 \\
    NDCG \& Ranking Accuracy        & 0.9938 & 0.00001 \\
    \midrule
    \midrule
    \multicolumn{3}{c}{ {Qwen1.5-1.8B-DRPO}}\\
    \midrule
    NDCG \& RM Win Rate             & 0.8441 & 0.000840 \\
    Ranking Accuracy \& RM Win Rate & 0.8069 & 0.01548 \\
    NDCG \& Ranking Accuracy        & 0.9767 & 0.00003 \\
    \bottomrule
    \end{tabular}
}
\end{center}
\end{table}

\section{GPT-4 Evaluation Details}  
% \addcontentsline{apc}{section}{\textnormal{F: GPT-4 Evaluation Details} } 
We use gpt-4-1106-preview for all our experiments. Table \ref{tab:gpt-4-prompt} presents our template for requesting GPT-4 during our GPT-4 evaluation. 

\input{tables/GPT4-template}

\section{Additional Qualitative Examples}
\addcontentsline{apc}{section}{\textnormal{I: Additional Qualitative Examples}}

In this section, we conduct more detailed qualitative experiments and verify the efficacy of our proposed methodology relative to competing approaches. In Table \ref{tab:example-qwen}, we use Qwen-1.5-1.8B as our base model, and train it using various methods. We present two examples to compare the responses generated by models trained with these methods. Additionally, we present the GPT-4 evaluation results for our example. The prompt in our example is sampled from the test split of the standard HH dataset. As table shows, our method can lead to more helpful, harmless and concise response.

Furthermore, we extend our method to fine-tune multi-modal large models and validate the effectiveness. We choose Qwen-VL-Chat as our base model, which is a popular multi-modal large model. We train it using various methods on VLFeedback dataset and compare its performance on MM-Vet benchmarks. In Table \ref{tab:example-qwen-vl}, we present two examples, each of which includes different responses generated by our models for the questions in the MM-Vet benchmark. As the table shows, the model trained using our method can generate higher-quality responses with fewer hallucinations compared to other methods. Furthermore, we provide more examples in Table \ref{tab:example-qwen-vl2}.

\input{tables/exmaple-response-qwen1.5}
\input{tables/example-response-qwen-vl}
