# Supplementary material for: Holistic Utility Preference Learning for Listwise Alignment
Source: arXiv:2410.18127 source file (2025-12-16)
Supplement: Supplementary file 2 [file appendix_proof.tex]

% \documentclass{article}
% % \documentclass{ctexart}

% % Language setting
% % Replace `english' with e.g. `spanish' to change the document language
% \usepackage[english]{babel}
% \usepackage{algorithm}
% \usepackage{algorithmic}
% %\textsl{}\setstretch{1.8}

% % Set page size and margins
% % Replace `letterpaper' with `a4paper' for UK/EU standard size
% \usepackage[letterpaper,top=2cm,bottom=2cm,left=3cm,right=3cm,marginparwidth=1.75cm]{geometry}
% % Useful packages
% \usepackage{amsmath}
% \usepackage{graphicx}
% \usepackage[colorlinks=true, allcolors=blue]{hyperref}

% \title{Direct Ranking Preference Optimization}
% \author{@caicai}

% \begin{document}
% \maketitle

% \section{lambdaloss}


% lambda loss function is :

% \[\begin{aligned}
% &\mathcal{L}_{\mathrm{lambda-loss}}(\theta)= 
% -\mathbb{E}_{x,\mathbf{y},\psi\sim\mathcal{D}}\left[\sum_{\psi_i>\psi_j}\Delta_{i,j}\log( \frac{1}{1+ e^{-(r_i-r_j) }})\right], \\
% &\begin{aligned}\text{where}\quad\Delta_{i,j}&=|G_i-G_j|\cdot|\frac{1}{D(\tau(i))}-\frac{1}{D(\tau(j))}|.\end{aligned}
% \end{aligned}
% \]

% rewrite the loss function as：
% \[
% \ell_\mathcal{D}(\theta) =-\frac{1}{n}\sum_{i=1}^{n}\sum_{j=0}^{K-1}\sum_{k=j+1}^{K-1} \Delta_{j,k}\log\frac{1}{1+e^{ - (r_j^i-r_k^i)}}
% \]
% \subsection{Lambdaloss in liner setting}

% In a linear environment setting $r_\theta(s,a)=\langle\theta,\phi(s,a)\rangle $ ,let $\begin{aligned}x_{jk}^i=\phi(s^i,a_j^i)-\phi(s^i,a_k^i)\end{aligned}$ ,then we can  rewrite the loss function as:
% \[
% \ell_\mathcal{D}(\theta) =-\frac{1}{n}\sum_{i=1}^{n}\sum_{j=0}^{K-1}\sum_{k=j+1}^{K-1} \Delta_{j,k}\log\frac{1}{1+\exp(- \langle\theta,x_{jk}^i\rangle) }.
% \]

% The gradient of the lambdaloss is

% \[\begin{aligned}\nabla\ell_D(\theta)&=-\frac1n\sum_{i=1}^n\sum_{j=0}^{K-1}\sum_{k=j+1}^{K-1}\Delta_{j,k} \frac{\exp(- \langle\theta,x_{jk}^i\rangle)}{1+\exp(- \langle\theta,x_{jk}^i\rangle) }\cdot x_{jk}^i.\end{aligned}\]


% The Hessian of the lambdaloss can be written as

% \[\begin{aligned}\nabla^2\ell_{\mathcal{D}}(\theta)&=\frac{1}{n}\sum_{i=1}^{n}\sum_{j=0}^{K-1}\sum_{k=j}^{K-1} \Delta_{j,k} \frac{\exp(- \langle\theta,x_{jk}^i\rangle)}{(1+\exp(- \langle\theta,x_{jk}^i\rangle) )^2}\cdot x_{jk}^i x_{jk}^{i\top}.\end{aligned}\]





% since the coefficients satisfy
% $$\begin{aligned}\frac{\exp(-\langle\theta,x^i_{\sigma_i(j)\sigma_i(k)})\rangle}{(1+\exp(-\langle\theta,x^i_{\sigma_i(j)\sigma_i(k)})\rangle)^2}\geq\frac1{2+\exp(2LB)+\exp(-2LB)}.\end{aligned}$$

% let $\gamma = \frac1{2+\exp(2LB)+\exp(-2LB)}$ We can verify that for any vector $v\in\mathbb{R}^K$ has:


% \begin{center}
%     \begin{aligned}
%         \begin{aligned}\upsilon^\top\nabla^2\ell_{\mathcal{D}}(\theta)v\end{aligned}& \begin{aligned}\geq\frac{\gamma}{n}v^\top\left(\sum_{i=1}^n\sum_{j=0}^{K-1}\sum_{k=j+1}^{K-1} \Delta_{j,k} x_{jk}^i x_{jk}^{i\top}}\right)v\end{aligned}  \\
%         &=\frac\gamma nv^\top\left(\sum_{i=1}^n\sum_{j=0}^{K-1}\sum_{k=j+1}^{K-1}\Delta_{j,k} x_{jk}^ix_{jk}^{i\top}\right)v \\
%         &= \frac{\gamma K(K-1)}{2} v^\top\Sigma_{\mathcal{D}}v \\
%         &= \frac{\gamma K(K-1)}{2} \|v\|_{\Sigma_{\mathcal{D}}}^2.
%     \end{aligned}

% \end{center}

% Here $\Sigma_{\mathcal{D}} = \frac2{K(K-1)n}\sum_{i=1}^n\sum_{j=0}^{K-1}\sum_{k=j+1}^{K-1} \Delta_{j,k} x_{jk}^ix_{jk}^{i\top} $ . let $\Delta=\hat \theta-\theta^{*}$ , one has


% \[\ell_{\mathcal{D}}(\theta^{\star}+\Delta)-\ell_{\mathcal{D}}(\theta^{\star})-\langle\nabla\ell_{\mathcal{D}}(\theta^{\star}),\Delta\rangle\leq-\langle\nabla\ell_{\mathcal{D}}(\theta^{\star}),\Delta\rangle.\]

% as for right side , we know $|\langle\nabla\ell_{\mathcal{D}}(\theta^\star),\Delta\rangle|\leq\|\nabla\ell_{\mathcal{D}}(\theta^\star)\|_{(\Sigma_{\mathcal{D}}+\lambda I)^{-1}}\|\Delta\|_{\Sigma_{\mathcal{D}}+\lambda I}\mathrm{~for~any~}\lambda>0.$ we have

% \begin{equation}
%     \begin{aligned}
%         \nabla\ell_D(\theta^{*})&=-\frac1n\sum_{i=1}^n\sum_{j=0}^{K-1}\sum_{k=j+1}^{K-1}\Delta_{j,k} \frac{\exp(- \langle \theta^{*},x_{jk}^i\rangle)}{1+\exp(- \langle\theta^{*},x_{jk}^i\rangle) } \cdot x_{jk}^i. \label{gradient_lambdaloss}
%     \end{aligned} 
% \end{equation}

% we set $X\in\mathbb{R}^{(nK(K-1)/2)\times d}$ , every row is \sqrt{\Delta_{j,k}} x_{jk}^i $$ , let  $V_{jk}^i$ is the random variable of the coefficient of $x^i_{jk}$ in \eqref{gradient_lambdaloss}

% \[V_{jk}^i=\begin{cases}\frac{\sqrt{\Delta_{j,k}} \exp(- \langle \theta^{*},x_{jk}^i\rangle)}{1+\exp(- \langle \theta^{*},x_{jk}^i\rangle)},&\text{ if }j<k\\-\frac{\sqrt{\Delta_{j,k}}}{1+ \exp(- \langle \theta^{*},x_{jk}^i\rangle)},&\text{ otherwise.}\end{cases}\] 

% Let $ \widetilde{V}_i \in\mathbb{R}^{K(K-1)/2} $ be the concatenated random vector of $\{V_{jk}^i\}_{0\leq j<k\leq K-1}$ , and $V\in\mathbb{R}^{nK(K-1)/2}$ be the concatenated random vector of $ {\widetilde{V}_i }_i^{n} $. $ \widetilde{V}_i $ is independent and $V$ is sub-Gaussian
% and $E[V] = 0$. since $ -\Delta_{jk} \leq V^i_{jk} \leq \Delta_{jk}$ ,$\sigma^2 \leq \sum_{j=0}^{K-1}\sum_{k=j+1}^{K-1}\Delta_{j,k} \leq \sum_{j=0}^{K-1} K \frac{G_j}{D_j} =  KN_g$. where $N_g = NDCG_{max}$ 

% then $\|\nabla\ell_{\mathcal{D}}(\theta^{\star})\|_{(\Sigma_{\mathcal{D}}+\lambda I)^{-1}}^{2}$ can be written as 

% \[
%     \|\nabla\ell_{\mathcal{D}}(\theta^{\star})\|_{(\Sigma_{\mathcal{D}}+\lambda I)^{-1}}^2=\frac1{n^2}V^{\top}X(\Sigma_{\mathcal{D}}+\lambda I)^{-1}X^{\top}V.
% \]

% Here, $\Sigma_{\mathcal{D}} = \frac2{K(K-1)n}X^{\top}X $ , $\lambda_{max}(X(\Sigma_{\mathcal{D}}+\lambda I)^{-1}X^{\top}) \leq \frac{K(K-1)n}2$ we can know $X(\Sigma_{\mathcal{D}}+\lambda I)^{-1}X^{\top}  \leq nK^2 I $ the upper bound the original term as

% \[
%     \|\nabla\ell_{\mathcal{D}}(\theta^{\star})\|_{(\Sigma_{\mathcal{D}}+\lambda I)^{-1}}^2 
%  \leq \frac{K^2}{n} \|V\| ^ 2 .
% \]
% By Bernstein’s inequality for sub-Gaussian random variables in quadratic form \cite{hsu2011tail}
% we know that with probability at least $1 - \delta$,
% \[
%     \|V\| ^ 2 \leq  C K N_g (d+\log^{\frac{1}{\delta}} )
% \]
% Thus altogether, we have

% \[
%      \|\nabla\ell_{\mathcal{D}}(\theta^{\star})\|_{(\Sigma_{\mathcal{D}}+\lambda I)^{-1}}^2 \leq
%      \frac{CK^4N_g}{nK} (d+\log^{\frac{1}{\delta}})
% \]

% \[
%     \gamma \|\Delta \|_{\Sigma_{\mathcal{D}}}  \leq \sqrt{ \frac{CN_g(d+\log^{\frac{1}{\delta}})}{nK} } \|\Delta \|_{\Sigma_{\mathcal{D}} + \lambda I}
% \]

% we can derive that with probability at least $1-\delta$

% \[\|\hat{\theta}-\theta^\star\|_{\Sigma_{\mathcal{D}}+\lambda I}\leq C\cdot\sqrt{\frac{N_g(d+\log^{\frac{1}{\delta}})}{Kn \gamma^2} +\lambda B^2}.\]



% \subsection{Lambdaloss in nonlinear setting}


% we can derive that with probability at least $1-\delta$
% \[\|\hat{\theta}-\theta^\star\|_{\Sigma_{\mathcal{D}}+\lambda I}\leq C_2\cdot\sqrt{\frac{N_g(d+\log^{\frac{1}{\delta}})}{Kn \gamma ^ {2}} + (\lambda + \frac{\alpha_2 N_g}{\gamma K}   + 2\alpha_1 \alpha_2 B )B^2}.\]

% Here, $\Sigma_{\mathcal{D}} = \frac2{K(K-1)n}\sum_{i=1}^n\sum_{j=0}^{K-1}\sum_{k=j+1}^{K-1} \Delta_{j,k} \nabla f_{\theta^{\star} jk}^{i} f_{\theta^{\star}}^{i\top} $ . 

% \subsection{ $MLE_2$ in nonlinear setting}

% we can derive that with probability at least $1-\delta$
% \[\|\hat{\theta}-\theta^\star\|_{\Sigma_{\mathcal{D}}+\lambda I}\leq C_2\cdot\sqrt{\frac{d+\log^{\frac{1}{\delta}}}{n \gamma^2} + (\lambda + \frac{\alpha_2 }{\gamma }   + 2\alpha_1 \alpha_2 B )B^2}.\]

% Here, $\Sigma_{\mathcal{D}} = \frac2{K(K-1)n}\sum_{i=1}^n\sum_{j=0}^{K-1}\sum_{k=j+1}^{K-1}  \nabla f_{\theta^{\star} jk}^{i} f_{\theta^{\star}}^{i\top} $ . 



% \begin{algorithm}
% 	%\textsl{}\setstretch{1.8}
% 	\renewcommand{\algorithmicrequire}{\textbf{Input:}}
% 	\renewcommand{\algorithmicensure}{\textbf{Output:}}

         
% 	\caption{Hard Odd Even Sort}
% 	\label{alg1}
% 	\begin{algorithmic}[1]

%             \REQUIRE{$ \boldsymbol{y} = (y_0,.... y_k) , \boldsymbol{x} = ( x_0, ... x_{k-1} ),x_i = (prompt, anser_i )$}
 
% 		\STATE Initialization: $ \boldsymbol{P} = I$ , $\boldsymbol{s} = (s_0, ... s_{k-1}) $, $s_i = log \frac{ \pi_{\theta}(x_i) }{\pi_{\mathrm{ref}}(x_i)} $
%             \REPEAT

%                 \STATE $P_{even} = I$ \\
%                 \FOR{$i \gets 0$ to $k-1$ by $2$}
%                     \IF{$s[i+1] > s[i]$}
%                         \STATE swap($s[i]$ ,$s[i+1]$)
%                         \STATE $P_{even} = P_{even} E_{i,i+1}$
%                     \ENDIF
                    
%                 \ENDFOR
%                 \\
%                 \STATE $P_{odd} = I$ \\
%                 \FOR{$i \gets 1$ to $k-1$ by $2$}
%                     \IF{$s[i] > s[i+1]$}
%                         % \STATE $a[i], a[i+1] \gets a[i+1], a[i]$
%                         \STATE swap($s[i]$ ,$s[i+1]$)
%                         \STATE $P_{odd} = P_{odd} E_{i,i+1}$
%                     \ENDIF
%                 \ENDFOR

%                 \STATE $ \boldsymbol{P} = P_{even} P_{odd} $ \\
                
%             \UNTIL $\boldsymbol{s} $ is sorted

% 		\ENSURE  sorted $\boldsymbol{s}$ , $\boldsymbol{P}$
  
% 	\end{algorithmic}  
% \end{algorithm}


% \begin{algorithm}
% 	%\textsl{}\setstretch{1.8}
% 	\renewcommand{\algorithmicrequire}{\textbf{Input:}}
% 	\renewcommand{\algorithmicensure}{\textbf{Output:}}
%         \renewcommand{\algorithmiccomment}[1]{\hfill $\triangleright$ #1}
        
% 	\caption{DRPO loss}
% 	\label{alg1}
% 	\begin{algorithmic}[1]

%             \REQUIRE{$ \boldsymbol{y} = (y_0,.... y_k) , \boldsymbol{x} = ( x_0, ... x_{k-1} ),x_i = (prompt, anser_i )$}
 
% 		\STATE Initialization: $ \boldsymbol{P} = I$ , $\boldsymbol{s} = (s_0, ... s_{k-1}) $, $s_i = log \frac{ \pi_{\theta}(x_i) }{\pi_{\mathrm{ref}}(x_i)} $, $\boldsymbol{d} = (d_0,... d_{k-1} )$,$d_i = log^{1+i}$
%             \STATE $even=0$ \\
%             \FOR{ $i = 1$ to $k$  }
            
%                 \STATE $\boldsymbol{P}^i = \boldsymbol{I} , j = even$ \\
                
%                 \FOR{$ j $ to $k-1$ by $2$}
%                     \STATE $\alpha = \sigma(s[j+1]-s[j])$
%                     % 
%                     \STATE $s[j] = (1-\alpha)s[j]  + \alpha s[j+1] $ \COMMENT{soft swap}
%                     \STATE $s[j+1] = \alpha s[j]  +(1- \alpha )s[j+1] $  

%                     \STATE $\boldsymbol{P}^i_{j,j} = 1-\alpha , \boldsymbol{P}^i_{j,j+1} = \alpha$
%                     \STATE $\boldsymbol{P}^i_{j+1,j} = \alpha , \boldsymbol{P}^i_{j+1,j+1} = 1 - \alpha$
                    
%                 \ENDFOR
%                 \STATE $even = ! even$ \\
%                 \STATE $\boldsymbol{P} = \boldsymbol{P} \boldsymbol{P}^i $ \\
                
%             \ENDFOR
            
%             \STATE $\ell = 1 - \frac{1}{iDCG} \frac{\boldsymbol{P}^\top \boldsymbol{y} }{ \boldsymbol{d} }  $ \\
		
%             \ENSURE  $\ell 
  
% 	\end{algorithmic} 
% \end{algorithm}

% % \begin{equation}
% %     E = mc^2
% %     \label{eq:\sig_func}
% % \end{equation}


%     % for i in xrange(1, len(a)-1, 2):
%     %     if a[i] > a[i+1]:
%     %        a[i], a[i+1] = a[i+1], a[i] # 交换
%     %        sorted = False
%     % # 处理偶-奇对
%     % for i in xrange(0, len(a)-1, 2):
%     %     if a[i] > a[i+1]:
%     %        a[i], a[i+1] = a[i+1], a[i] # 交换
%     %        sorted = False
% \usepackage{algorithm}
% \usepackage{algorithmicx}
% \usepackage{algpseudocode}



% $K= 2 $  Case:

% $$\ell = -\frac{1}{n} \sum_{i=1}^n  \frac{1}{iDCG} (y_1 - y_2)(\frac{1}{d_1} - \frac{1}{d_2}) \sigma(s_1 - s_2)$$



% \bibliographystyle{plain}
% \bibliography{refs}


% \end{document}
