# Supplementary material for: Holistic Utility Preference Learning for Listwise Alignment
Source: arXiv:2410.18127 source file (2025-12-16)
Supplement: Supplementary file 3 [file experimental_detail.tex]

\section{Construction the Ranking Preference Data}
% \addcontentsline{apc}{section}{\textnormal{D: Construction the Ranking Preference Data.} } 
\label{appendix:rankhh}
% Datasets. Anthropic’s Helpful and Harmless (HH) [Bai et al., 2022] contains 161k/8.5k train-245
% ing/test samples. Each sample consists of a prompt and a pair of responses (chosen and reject),246
% where “chosen" represents the preferred response and “reject" represents the less preferred response.247
% We also generate additional responses for each prompt and rate each response using a reward model248
% DeBERTa2, resulting in ranking preference data of a list size K = 8. For more details, please refer249
% to Appendix C.

\textbf{HH Dataset.} To construct ranking preference data based on \textbf{HH} dataset, we first supervised fine-tune(SFT) the Qwen1.5-4B model with \textbf{HH} dataset. Subsequently, we sample $K=6$ responses for each prompt $x^i$ in \textbf{HH} dataset using trained SFT model (Qwen1.5-4B) with parameter $temperature = 0.7, top\_k = 40$. We combine the sampled data and the original pairwise data to obtain the $K=8$ responses. We then score each response with a reward model $R$. In our work, we use the RM-Deberta-v3-large-v2\footnotemark[\value{footnote}] model as our reward model, which is based on the DeBERTaV3 \cite{DBLP:conf/iclr/HeLGC21}, subsequently trained on the HH dataset. 

Specifically, following \cite{liu2024lipo}, we compute the score $s^i_j$ of each response $y^i_j$ with respect to the prompt $x^i$ as follows:
\begin{equation*}
s^i_{j} = \frac{1}{K} \sum_{l=1}^{K} \frac{e^{R(x^{i},y^i_{j})}}{e^{R(x^{i},y^i_{j})} + e^{R(x^{i},y^i_{l})}}, \text{where} ~ R ~ \text{is a reward model}.
\label{sig_func}
\end{equation*}

Based on the discussion above, we can construct our ranking preference dataset as $D = \{x^i, \mathbf{y}^i, \mathbf{s}^i\}_{i=1}^N$, where $\mathbf{y}^i = (y^i_1,...,y^i_K)$ and $ \mathbf{s}^i 
= (s^i_1,...,s^i_K)$. To support conducting an ablation study on the size $K$ of the ranking preference dataset, we also split this dataset of size $K=8$ into three subsets, each with sizes $K=2$, $K=4$, and $K=6$, respectively. We also provide an example of our ranking preference dataset as shown in Table \ref{tab:example-hhrank}.

\textbf{UltraFeedback Dataset.} This dataset itself contains four responses and corresponding scores, which can be directly used to construct a ranking preference dataset of size $K=4$. We simply normalize these scores to the range $[0,1]$.

\textbf{VLFeedback Dataset.} Similar to the UltraFeedback Dataset, this dataset can be used directly as a ranking preference dataset of size $K=4$. We simply normalize these scores to the range $[0,1]$.

\input{tables/example-rankhh}
