# Supplementary material for: Holistic Utility Preference Learning for Listwise Alignment
Source: arXiv:2410.18127 source file (2025-12-16)
Supplement: Supplementary file 5 [file reletaed_works.tex]

% \section{Detail Limitations}
% \addcontentsline{apc}{section}{\textnormal{B: Limitations}}

% In conducting our experiments, we adhere to benchmarks that are widely recognized and routinely utilized in the literature on human preference alignment. It is important to note, however, that despite our best efforts, there remain certain unavoidable limitations that merit consideration. In the process of constructing a ranking preference dataset, we employ a reward model to serve as a proxy for human evaluations. While the reward model we employ achieves a high level of accuracy, it is important to acknowledge that there might still be subtle discrepancies when compared to human evaluations. In the future, we are also interested in exploring more high-quality reward models as proxies for human evaluations. 

\section{Detailed Sorting Process in Sorting Networks}
\label{sec:sorting_detail}

This work leverages the odd-even sorting network algorithm. As depicted in Figure \ref{fig:diff_sort}, an ordered sequence of $K$ elements can be achieved through a $K\text{-layer}$ sorting network. Each layer of the odd-even sorting network operates by comparing and swapping \textit{adjacent elements} at either odd or even indices, thereby organizing them in a desired order. The process alternates between odd and even stages. During the odd stage, all pairs of elements at odd indices (i.e., positions 1 and 2, 3 and 4, 5 and 6, etc.) are compared and swapped if necessary according to the desired order. In the even stage, all pairs of elements at even indices (i.e., positions 2 and 3, 4 and 5, 6 and 7, etc.) are compared and swapped according to the desired order.

To illustrate this mechanism, consider an unordered sequence $(10, 2, 4, 8)$ with length $K=4$ that we wish to arrange in descending order. The sorting process proceeds through alternating phases as follows:

\begin{itemize}
\item The first iteration (even phase) begins with indices $0$ and $2$, corresponding to values $(10, 4)$. These elements are compared with their subsequent elements $(2, 8)$ respectively. Since $10 > 2$ satisfies the descending order requirement, no swap is needed for the first pair. However, $4 < 8$ violates the descending order requirement, so $4$ and $8$ are swapped. This phase yields an intermediate sequence $(10, 2, 8, 4)$. 

\item The second iteration (odd phase) focuses on indices $1$ and $3$, corresponding to elements $(2, 8)$. The element $2$ is compared with its subsequent element $8$, and since $2 < 8$, they are swapped. The element at index $3$ has no subsequent element for comparison, thus remaining unchanged. This phase transforms the sequence to $(10, 8, 2, 4)$. 

\item In the third iteration (even phase), indices $0$ and $2$ are examined. At index $0$, since $10 > 8$, no swap is needed. At index $2$, comparing $2$ with $4$, since $2 < 4$, they are swapped. Upon reaching a sequence satisfying the descending-order property $(10, 8, 4, 2)$, the algorithm terminates.
\end{itemize}

\begin{wrapfigure}{h}{0.32\textwidth}
    \vspace{-1em}
    \centering
    \includegraphics[width=0.32\columnwidth]{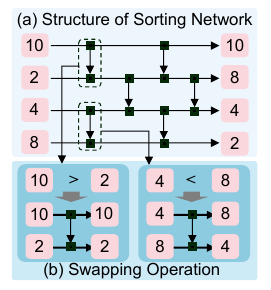}
    % \vspace{-0.1em}
    \caption{Sort $\mathbf{s}=(10,2,4,8)$ in descending order using a sorting network. (a) The structure of the sorting network; (b) the swapping operation in the first layer. }
    \label{fig:diff_sort}
    \vspace{-0.25em}
\end{wrapfigure}

As illustrated in Section \ref{sec:diff_swap_op}, this sorting operation can also be represented using permutation matrices. In our sorting process, the corresponding permutation matrices for each iteration are:
\begin{equation*}
    \mathbf{P}_1 = \begin{bmatrix}
    1 & 0 & 0 & 0 \\
    0 & 1 & 0 & 0 \\
    0 & 0 & 0 & 1 \\
    0 & 0 & 1 & 0
    \end{bmatrix}, \quad
    \mathbf{P}_2 = \begin{bmatrix}
    1 & 0 & 0 & 0 \\
    0 & 0 & 1 & 0 \\
    0 & 1 & 0 & 0 \\
    0 & 0 & 0 & 1
    \end{bmatrix}, \quad
    \mathbf{P}_3 = \begin{bmatrix}
    1 & 0 & 0 & 0 \\
    0 & 1 & 0 & 0 \\
    0 & 0 & 0 & 1 \\
    0 & 0 & 1 & 0
    \end{bmatrix}
\end{equation*}
Therefore, starting with initial sequence $\mathbf{s}_0 = [10, 2, 4, 8]^\top$, each layer's result can be represented through matrix multiplication: $\mathbf{s}_1 = \mathbf{P}_1^{\top} \cdot \mathbf{s}_0, \quad \mathbf{s}_2 = \mathbf{P}_2^{\top} \cdot \mathbf{s}_1, \quad \mathbf{s}_3 = \mathbf{P}_3^{\top} \cdot \mathbf{s}_2$. We can also obtain the complete sorting process's permutation matrix as follows:
\begin{equation*}
    \mathbf{P} = \mathbf{P}_1 \cdot \mathbf{P}_2 \cdot \mathbf{P}_3 = \begin{bmatrix}
    1 & 0 & 0 & 0 \\
    0 & 0 & 1 & 0 \\
    0 & 0 & 0 & 1 \\
    0 & 1 & 0 & 0
    \end{bmatrix}
\end{equation*}
The final ordered sequence is therefore given by:
\begin{equation*}
    \mathbf{s}_{\text{order}} = \mathbf{P}^{\top} \cdot \mathbf{s} = [10, 8, 4, 2]^\top.
\end{equation*}
